# Supplementary material for: Broadband Absorption in Cadmium Telluride Thin-Film Solar Cells via Composite Light Trapping Techniques
Source: arXiv:2502.20539 source file (2025-02-27)
Supplement: Supplementary file 1 [file supplement.pdf]

# Supplementary Information:

## Broadband Absorption in Cadmium Telluride Thin-Film Solar Cells via Composite Light-Trapping Techniques

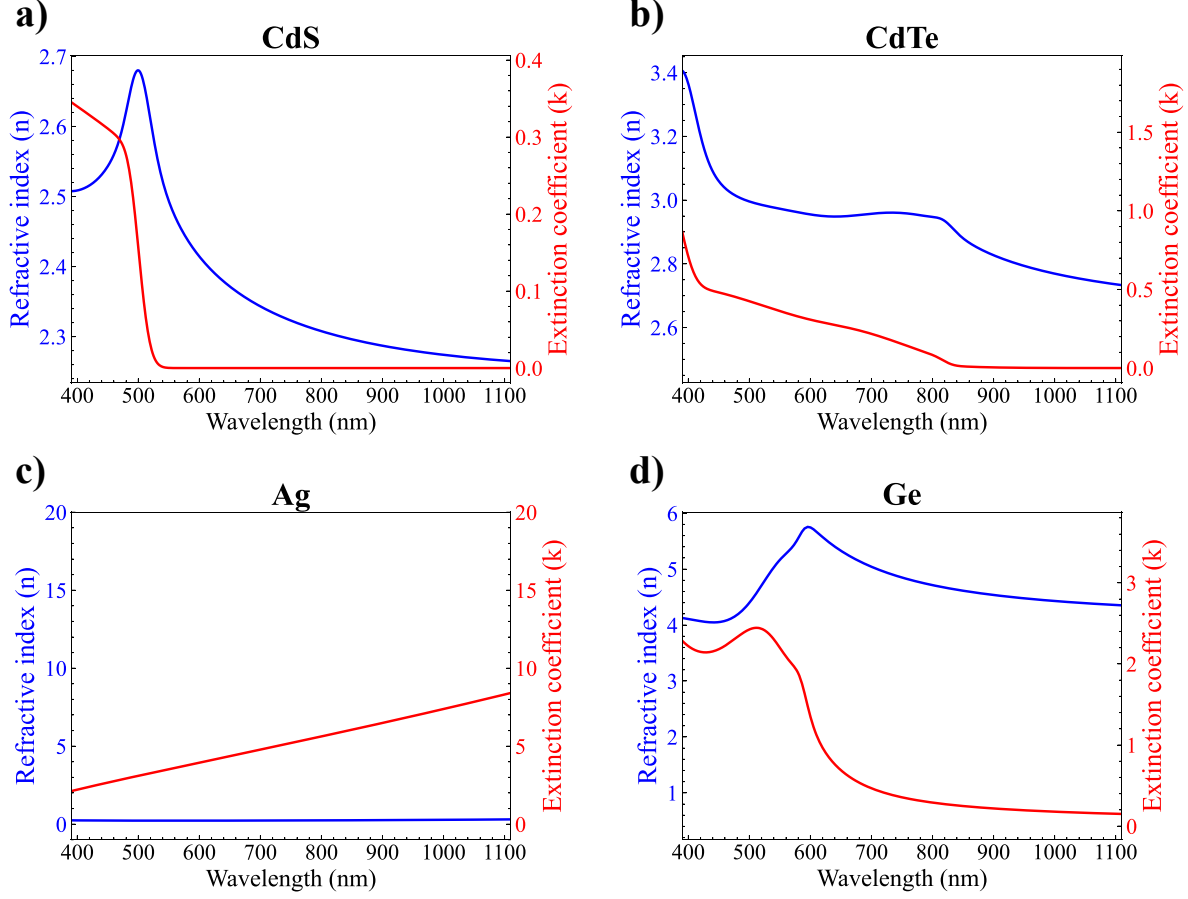

FIG. S1. Refractive index ( $n$ ) and extinction coefficient ( $k$ ) spectra of (a) CdS (b) CdTe, (c) Ag, and (d) Ge.

TABLE S1. CHARGE parameters for electrical simulations.

| Parameters      | Description                                          | CdTe                                          | CdS                                           |
|-----------------|------------------------------------------------------|-----------------------------------------------|-----------------------------------------------|
| $E_g$           | Bandgap                                              | 1.61 eV                                       | 2.56 eV                                       |
| $\epsilon_r$    | Relative permittivity                                | 10.2                                          | 10                                            |
| $\mu_n$         | Electron mobility                                    | $1050 \text{ cm}^2\text{V}^{-1}\text{s}^{-1}$ | $340 \text{ cm}^2\text{V}^{-1}\text{s}^{-1}$  |
| $\mu_p$         | Hole mobility                                        | $100 \text{ cm}^2\text{V}^{-1}\text{s}^{-1}$  | $340 \text{ cm}^2\text{V}^{-1}\text{s}^{-1}$  |
| $m_n$           | Effective mass of electron                           | $0.11/m_e$                                    | $0.21/m_e$                                    |
| $m_h$           | Effective mass of hole                               | $0.76/m_e$                                    | $1.015/m_e$                                   |
| $N_a$           | Uniform acceptor doping concentration                | $2 \times 10^{14} \text{ cm}^{-3}$            | -                                             |
| $N_d$           | Uniform donor doping concentration                   | -                                             | $1.1 \times 10^{18} \text{ cm}^{-3}$          |
| $\tau_n$        | Trap-assisted (Rsrh) electron recombination lifetime | $1 \times 10^{-6} \text{ s}$                  | $1 \times 10^{-6} \text{ s}$                  |
| $\tau_p$        | Trap-assisted (Rsrh) hole recombination lifetime     | $1 \times 10^{-6} \text{ s}$                  | $1 \times 10^{-6} \text{ s}$                  |
| $C_{n,Auger}$   | Auger recombination of electrons at 300 K            | $1 \times 10^{-34} \text{ cm}^6\text{s}^{-1}$ | $1 \times 10^{-34} \text{ cm}^6\text{s}^{-1}$ |
| $C_{p,Auger}$   | Auger recombination of holes at 300 K                | $1 \times 10^{-34} \text{ cm}^6\text{s}^{-1}$ | $1 \times 10^{-34} \text{ cm}^6\text{s}^{-1}$ |
| $C_{Radiative}$ | Radiative recombination coefficient at 300 K         | $1 \times 10^{-20} \text{ cm}^3\text{s}^{-1}$ | $1 \times 10^{-20} \text{ cm}^3\text{s}^{-1}$ |

\* $m_e$  = rest mass of electron

TABLE S2: Photovoltaic parameters i.e. short-circuit current density ( $J_{sc}$ ), open-circuit voltage ( $V_{oc}$ ), fill factor (FF), and power conversion efficiency (PCE), as a function of nanocone texture base diameter ( $d_{cone}$ ) and height ( $h_{cone}$ ). The  $J_{sc}$ ,  $V_{oc}$ , fill factor, and PCE for bare CdTe TFSCs are 24.33 mA/cm<sup>2</sup>, 978 mV, 0.6455, and 15.36%, respectively.

| Nanocone base diameter (nm) | Nanocone height (nm) | $J_{sc}$ (mA/cm <sup>2</sup> ) | $V_{oc}$ (mV) | Fill Factor | PCE (%) |
|-----------------------------|----------------------|--------------------------------|---------------|-------------|---------|
| 300                         | 50                   | 25.21                          | 929.6         | 0.8172      | 19.15   |
|                             | 100                  | 26.67                          | 925           | 0.8259      | 20.37   |
|                             | 150                  | 28.03                          | 925.8         | 0.8287      | 21.5    |
|                             | 200                  | 28.95                          | 926.1         | 0.8301      | 22.25   |
|                             | 250                  | 29.42                          | 926.1         | 0.8313      | 22.65   |
|                             | 300                  | 29.66                          | 925.9         | 0.8323      | 22.86   |
|                             | 350                  | 29.77                          | 925.8         | 0.834       | 22.99   |
|                             | 400                  | 29.81                          | 925.7         | 0.8355      | 23.05   |
| 400                         | 50                   | 25.1                           | 930.3         | 0.8156      | 19.04   |
|                             | 100                  | 26.44                          | 925           | 0.8242      | 20.16   |
|                             | 150                  | 27.97                          | 926           | 0.8268      | 21.41   |
|                             | 200                  | 29.18                          | 926.7         | 0.8282      | 22.39   |
|                             | 250                  | 29.88                          | 927.1         | 0.8292      | 22.97   |
|                             | 300                  | 30.27                          | 927           | 0.8307      | 23.31   |
|                             | 350                  | 30.58                          | 927           | 0.8317      | 23.58   |
|                             | 400                  | 30.74                          | 926.7         | 0.8341      | 23.76   |
| 500                         | 50                   | 25.12                          | 930.4         | 0.8149      | 19.04   |
|                             | 100                  | 26.4                           | 924.9         | 0.8232      | 20.1    |
|                             | 150                  | 26.43                          | 924.5         | 0.8247      | 20.15   |
|                             | 200                  | 29.31                          | 926.8         | 0.8258      | 22.43   |
|                             | 250                  | 30.47                          | 927.6         | 0.8263      | 23.35   |
|                             | 300                  | 31.14                          | 927.9         | 0.8273      | 23.9    |
|                             | 350                  | 31.71                          | 928.4         | 0.8275      | 24.36   |
|                             | 400                  | 31.85                          | 928.2         | 0.8291      | 24.51   |
| 600                         | 50                   | 25.01                          | 930.2         | 0.815       | 18.96   |
|                             | 100                  | 26.06                          | 924.8         | 0.8218      | 19.8    |
|                             | 150                  | 27.39                          | 925.4         | 0.8235      | 20.87   |
|                             | 200                  | 28.98                          | 926.4         | 0.8233      | 22.1    |
|                             | 250                  | 30.04                          | 927.1         | 0.824       | 22.95   |
|                             | 300                  | 31                             | 927.8         | 0.8246      | 23.72   |
|                             | 350                  | 31.69                          | 928.3         | 0.8252      | 24.28   |
|                             | 400                  | 32.09                          | 928.7         | 0.8259      | 24.62   |
| 700                         | 50                   | 25.01                          | 930           | 0.8128      | 18.9    |
|                             | 100                  | 25.87                          | 925.6         | 0.8213      | 19.66   |
|                             | 150                  | 26.98                          | 925           | 0.8225      | 20.53   |
|                             | 200                  | 28.17                          | 925.5         | 0.8228      | 21.45   |
|                             | 250                  | 29.05                          | 926.1         | 0.8232      | 22.15   |
|                             | 300                  | 29.74                          | 926.6         | 0.8242      | 22.71   |
|                             | 350                  | 30.52                          | 927           | 0.825       | 23.34   |
|                             | 400                  | 31.1                           | 927.7         | 0.8254      | 23.81   |
| 800                         | 50                   | 25.12                          | 930           | 0.8126      | 18.99   |
|                             | 100                  | 26.13                          | 925.9         | 0.82        | 19.84   |
|                             | 150                  | 27.34                          | 925.5         | 0.8205      | 20.76   |
|                             | 200                  | 28.4                           | 926.1         | 0.8205      | 21.58   |
|                             | 250                  | 29.47                          | 926.9         | 0.8207      | 22.42   |
|                             | 300                  | 30.16                          | 927.4         | 0.8216      | 22.98   |
|                             | 350                  | 30.89                          | 927.7         | 0.8227      | 23.58   |
|                             | 400                  | 31.21                          | 928           | 0.8241      | 23.87   |
| 900                         | 50                   | 24.89                          | 929.9         | 0.8132      | 18.82   |
|                             | 100                  | 25.43                          | 925.5         | 0.8212      | 19.33   |
|                             | 150                  | 26.28                          | 924.7         | 0.8221      | 19.98   |
|                             | 200                  | 27.1                           | 924.6         | 0.8231      | 20.62   |
|                             | 250                  | 28.13                          | 925.2         | 0.8227      | 21.41   |
|                             | 300                  | 28.88                          | 925.9         | 0.8229      | 22      |
|                             | 350                  | 29.89                          | 926.8         | 0.8225      | 22.79   |
|                             | 400                  | 30.62                          | 927.5         | 0.8225      | 23.36   |

TABLE S3: Photovoltaic parameters i.e. short-circuit current density ( $J_{sc}$ ), open-circuit voltage ( $V_{oc}$ ), fill factor (FF), and power conversion efficiency (PCE), as a function of Ge NP diameter ( $d_{Ge}$ ) and height ( $z_{Ge}$ ). The  $J_{sc}$ ,  $V_{oc}$ , fill factor, and PCE for bare CdTe TFSCs are 24.33 mA/cm<sup>2</sup>, 978 mV, 0.6455, and 15.36%, respectively.

| Nanoparticle diameter (nm) | Nanoparticle position (nm) | $J_{sc}$ (mA/cm <sup>2</sup> ) | $V_{oc}$ (mV) | Fill Factor | PCE (%) |
|----------------------------|----------------------------|--------------------------------|---------------|-------------|---------|
| 50                         | 500                        | 32.15                          | 928.8         | 0.8259      | 24.66   |
|                            | 600                        | 32.10                          | 928.7         | 0.8259      | 24.62   |
|                            | 700                        | 32.12                          | 928.7         | 0.8259      | 24.64   |
|                            | 800                        | 32.14                          | 928.7         | 0.8259      | 24.65   |
|                            | 900                        | 32.13                          | 928.7         | 0.8259      | 24.65   |
|                            | 1000                       | 32.14                          | 928.7         | 0.8259      | 24.65   |
|                            | 1100                       | 32.13                          | 928.7         | 0.8259      | 24.65   |
|                            | 1200                       | 32.14                          | 928.7         | 0.8258      | 24.65   |
| 100                        | 500                        | 32.28                          | 929.0         | 0.8268      | 24.80   |
|                            | 600                        | 32.07                          | 928.8         | 0.8272      | 24.64   |
|                            | 700                        | 32.22                          | 928.9         | 0.8266      | 24.73   |
|                            | 800                        | 32.21                          | 928.9         | 0.8265      | 24.73   |
|                            | 900                        | 32.19                          | 928.8         | 0.8264      | 24.71   |
|                            | 1000                       | 32.18                          | 928.8         | 0.8261      | 24.69   |
|                            | 1100                       | 32.27                          | 928.9         | 0.8256      | 24.74   |
|                            | 1200                       | 32.17                          | 928.8         | 0.8256      | 24.67   |
| 150                        | 500                        | 32.77                          | 929.8         | 0.8313      | 25.33   |
|                            | 600                        | 32.45                          | 929.4         | 0.8306      | 25.05   |
|                            | 700                        | 32.55                          | 929.4         | 0.8293      | 25.09   |
|                            | 800                        | 32.39                          | 929.2         | 0.8283      | 24.93   |
|                            | 900                        | 32.56                          | 929.3         | 0.8273      | 25.03   |
|                            | 1000                       | 32.56                          | 929.2         | 0.8262      | 25.00   |
|                            | 1100                       | 32.62                          | 929.2         | 0.8250      | 25.00   |
|                            | 1200                       | 32.75                          | 929.2         | 0.8232      | 25.05   |
| 200                        | 500                        | 33.53                          | 931.0         | 0.8371      | 26.13   |
|                            | 600                        | 33.82                          | 931.1         | 0.8343      | 26.27   |
|                            | 700                        | 33.67                          | 930.9         | 0.8326      | 26.10   |
|                            | 800                        | 33.26                          | 930.2         | 0.8306      | 25.70   |
|                            | 900                        | 32.69                          | 929.5         | 0.8290      | 25.19   |
|                            | 1000                       | 33.19                          | 929.9         | 0.8267      | 25.51   |
|                            | 1100                       | 33.27                          | 929.7         | 0.8241      | 25.49   |
|                            | 1200                       | 33.68                          | 929.8         | 0.8188      | 25.64   |
| 250                        | 500                        | 34.47                          | 932.2         | 0.8385      | 26.94   |
|                            | 600                        | 34.49                          | 932.0         | 0.8368      | 26.90   |
|                            | 700                        | 34.40                          | 931.8         | 0.8348      | 26.75   |
|                            | 800                        | 33.67                          | 930.8         | 0.8332      | 26.11   |
|                            | 900                        | 32.94                          | 929.8         | 0.8303      | 25.44   |
|                            | 1000                       | 33.53                          | 930.3         | 0.8278      | 25.82   |
|                            | 1100                       | 34.03                          | 930.4         | 0.8233      | 26.07   |
|                            | 1200                       | 33.85                          | 929.9         | 0.8180      | 25.75   |
| 300                        | 500                        | 35.38                          | 933.2         | 0.8406      | 27.76   |
|                            | 600                        | 35.02                          | 932.7         | 0.8396      | 27.42   |
|                            | 700                        | 34.51                          | 932.0         | 0.8372      | 26.93   |
|                            | 800                        | 33.64                          | 930.9         | 0.8356      | 26.17   |
|                            | 900                        | 34.01                          | 931.1         | 0.8325      | 26.36   |
|                            | 1000                       | 34.02                          | 930.8         | 0.8285      | 26.24   |
|                            | 1100                       | 34.11                          | 930.5         | 0.8234      | 26.13   |
|                            | 1200                       | 34.37                          | 930.2         | 0.8154      | 26.07   |

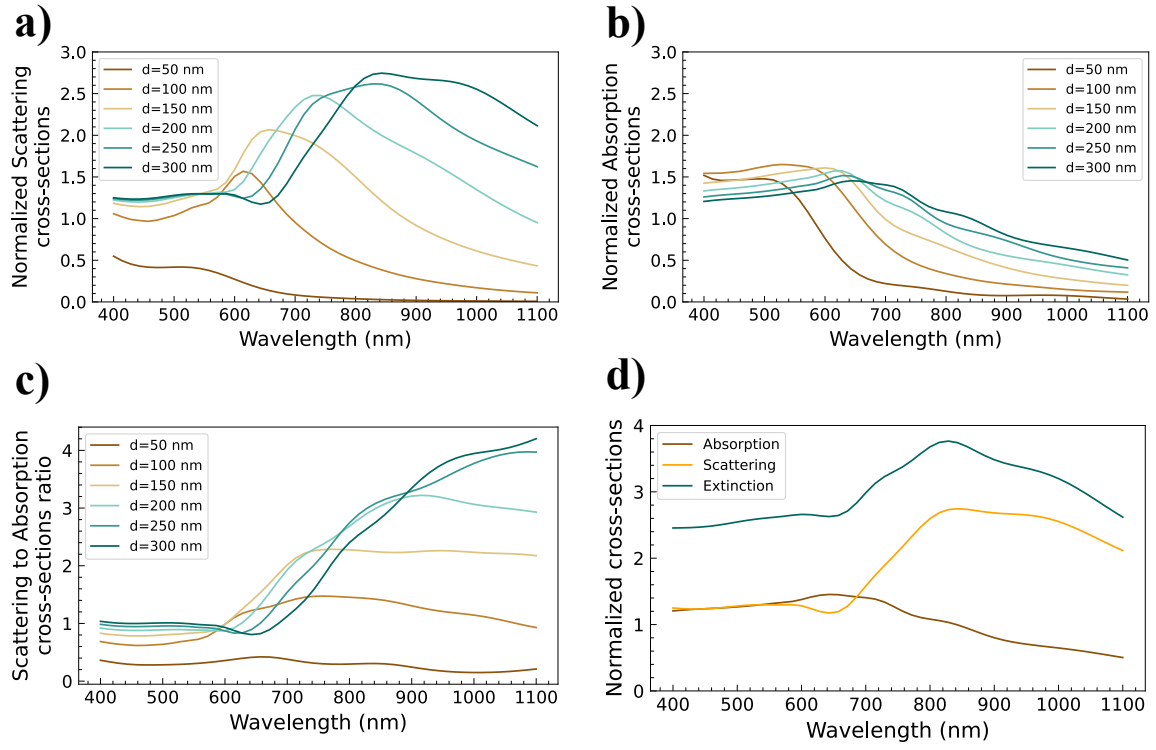

FIG. S2. (a) Mie analysis for Ge NP showing (a) Normalized scattering cross-sections for  $d = 50, 100, 150, 200, 250, 300$  nm, (b) Normalized absorption cross-sections for  $d = 50, 100, 150, 200, 250, 300$  nm, (c) Scattering to absorption cross-sections for  $d = 50, 100, 150, 200, 250, 300$  nm, (d) Normalized absorption, scattering, extinction cross-section for  $d = 300$  nm.

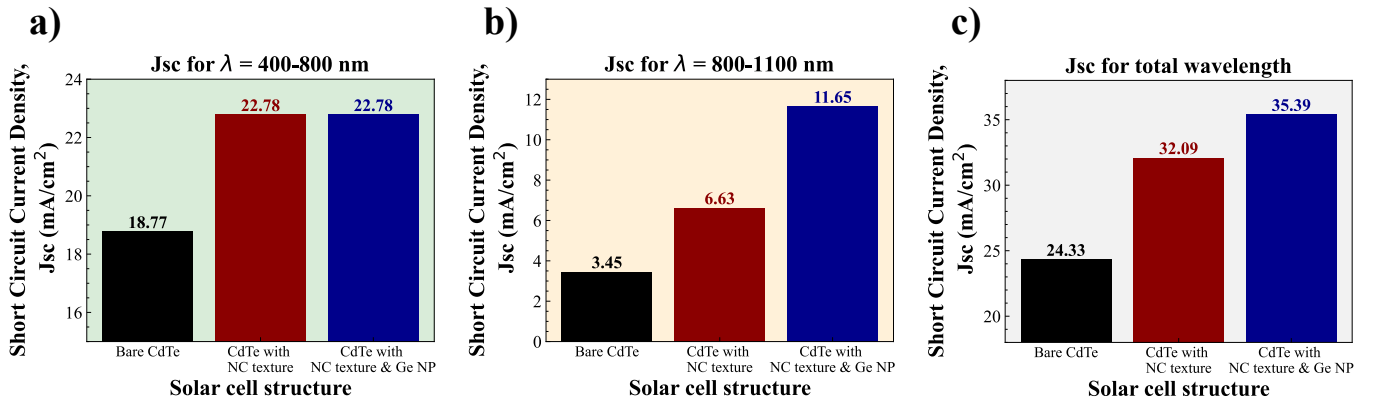

FIG. S3.  $J_{sc}$  for 400-800 nm wavelength range, (b)  $J_{sc}$  for 800-1100 nm wavelength range, (c)  $J_{sc}$  for the total wavelength (400-1100 nm) range of bare CdTe TFSCs, NC textured CdTe and NC textured CdTe with Ge NP.

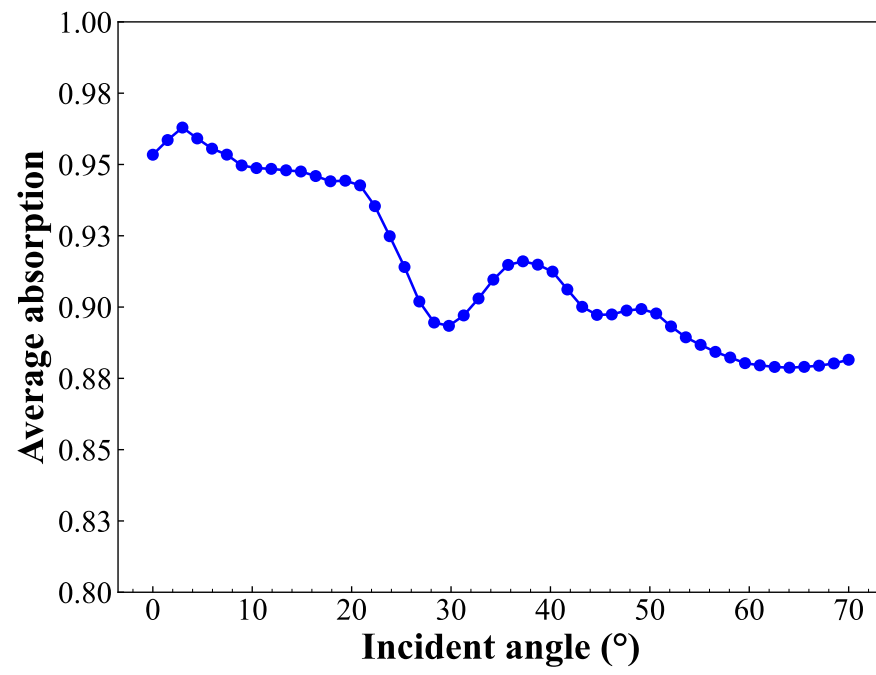

FIG. S4. Average absorption of NC textured CdTe with embedded Ge NP structure as a function of incident angle variation of 0° to 70°.
